# Supplementary material for: Sharp bounds of constants in Poincare type inequalities for polygonal domains
Source: arXiv:1504.03166 source file (2016-02-04)
Supplement: Supplementary file 1 [file appendix.tex]

\newpage

\newpage
\section{Appendix}
For convenience, we collect in this part the graphics
cited in Section \ref{eq:numerial-tests-2d}
and \ref{eq:numerial-tests-3d}.

%\newpage
%-------------------------------------------------------------------------------------------%
% \CPT with upper bounds
%--------------------------------------------------------------------------------------------%

\begin{figure}[!ht]
	\centering
	\subfloat[$\rho = \tfrac{\sqrt{3}}{2}$]{
  \includegraphics[scale=0.95]{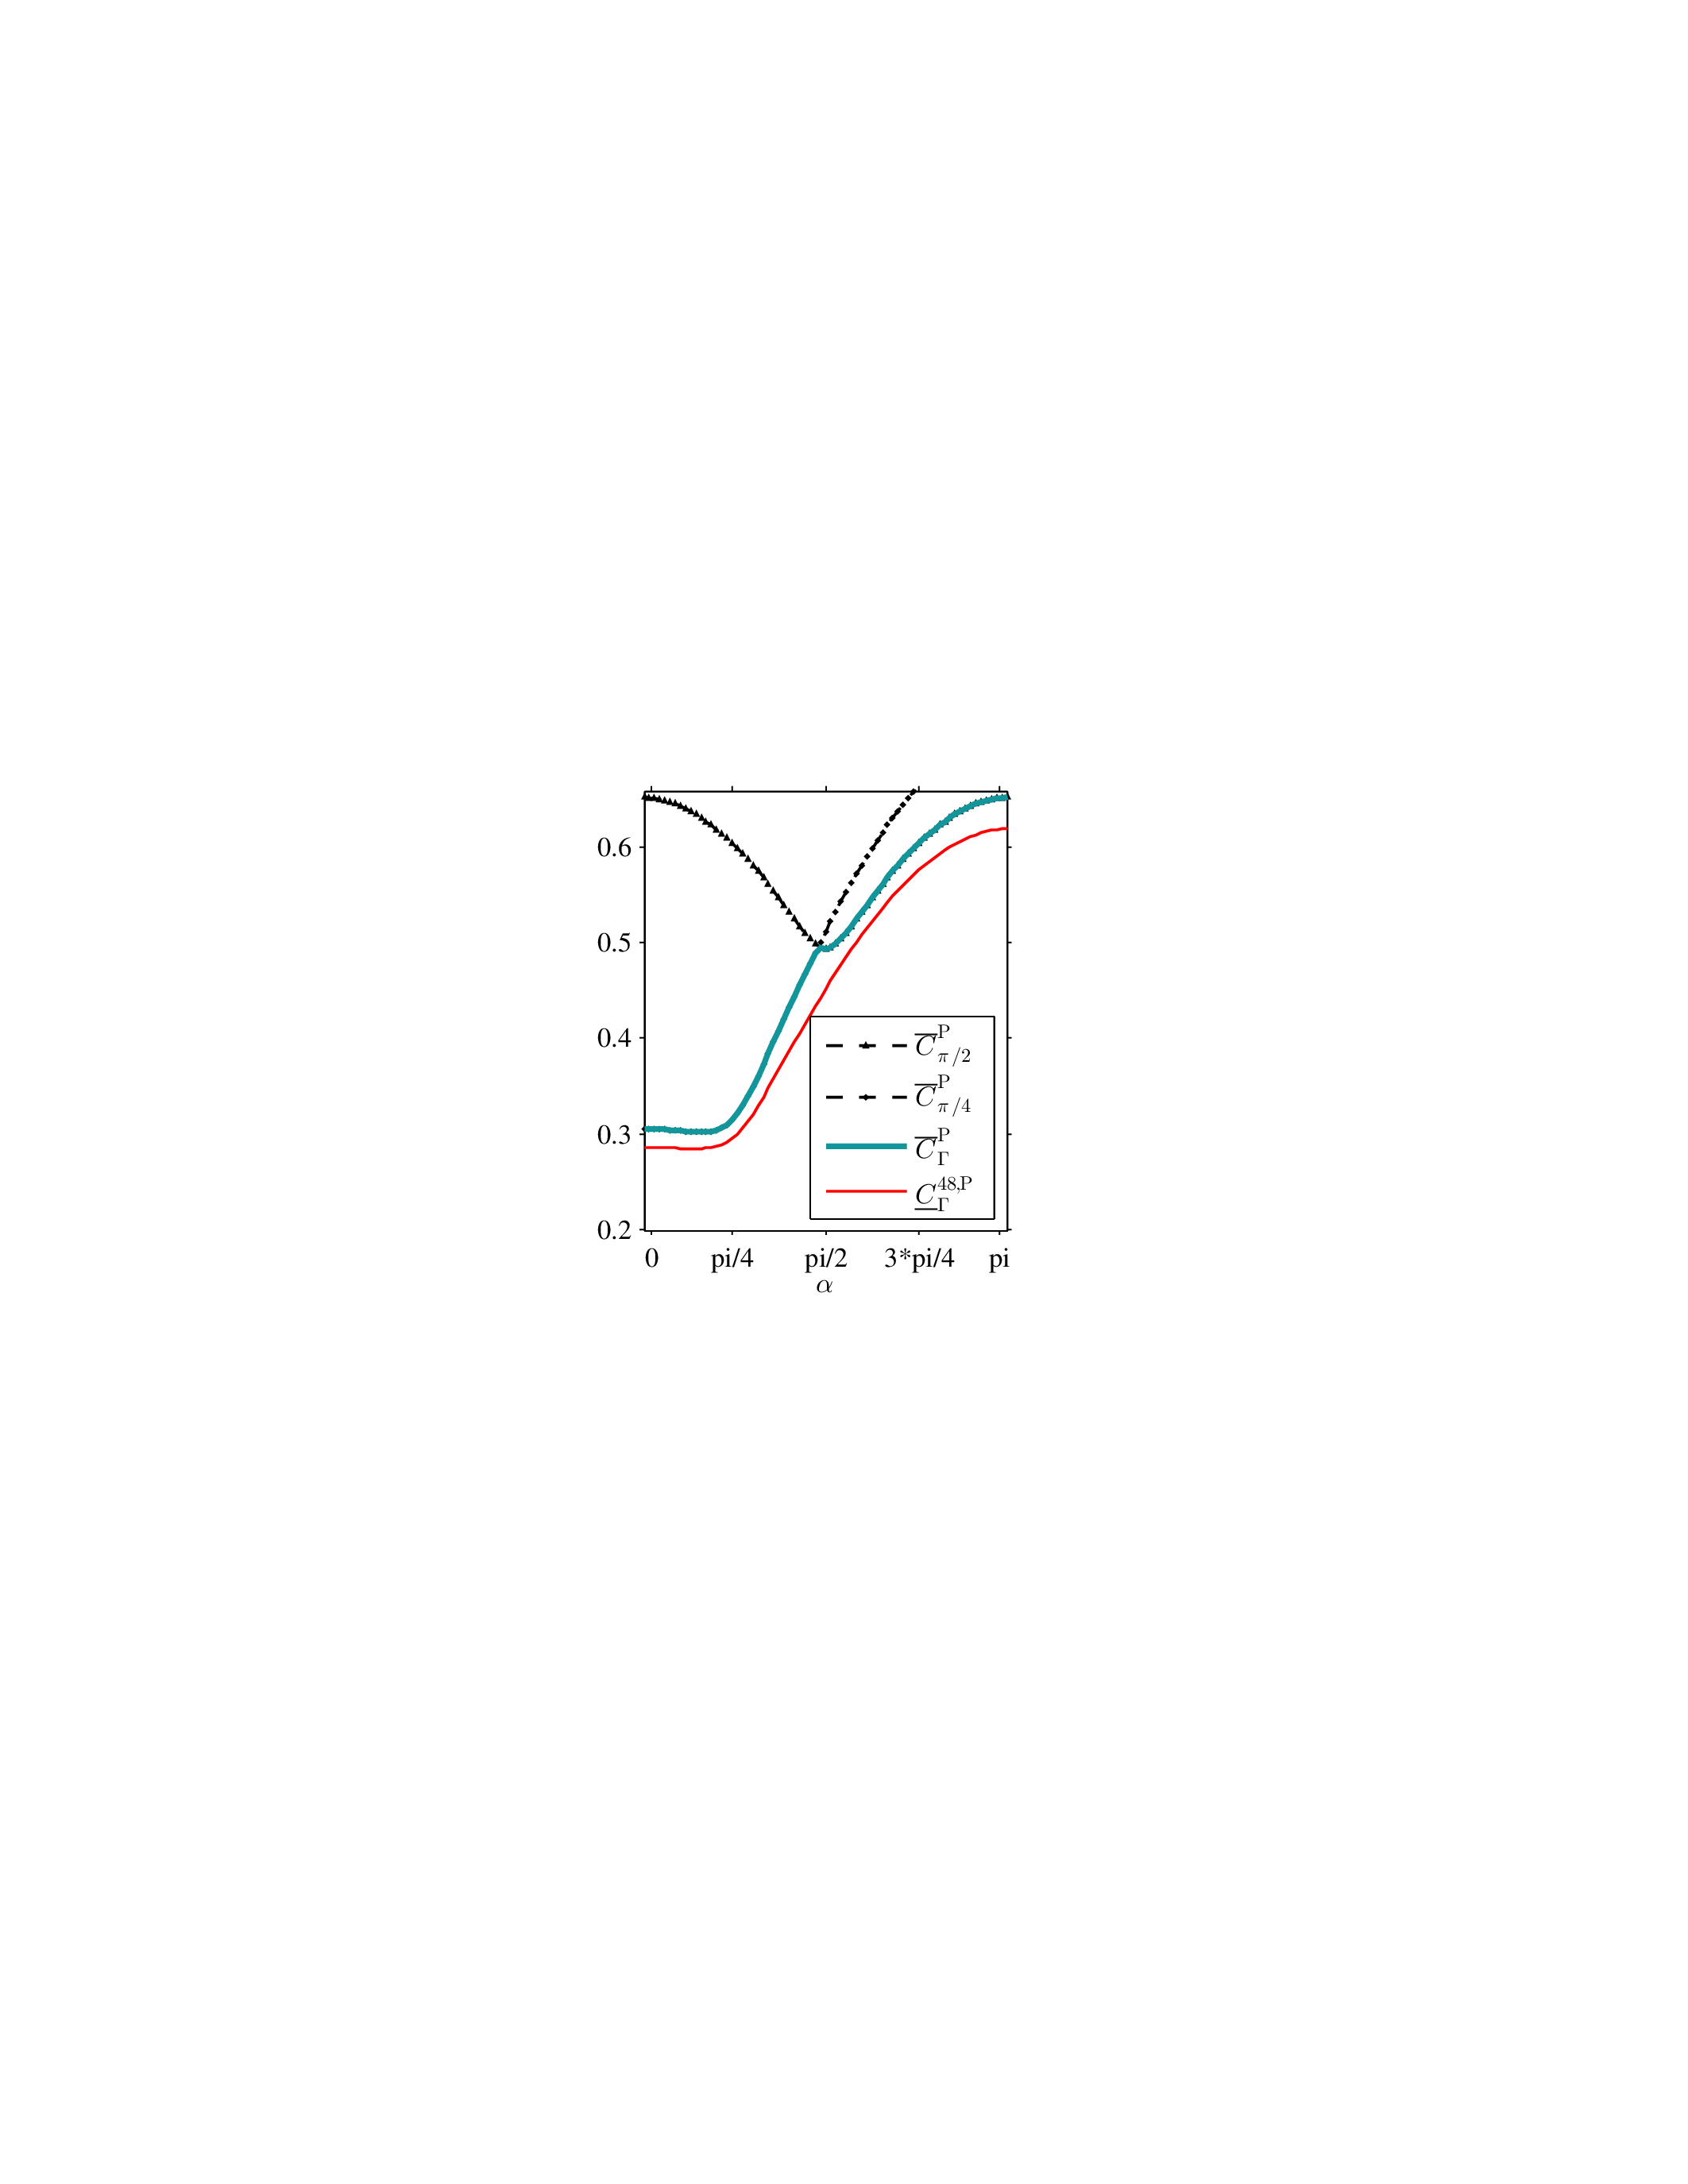}
	\label{fig:2d-cpt-rho-sqrt3-2}}
	\quad
	\subfloat[$\rho = \tfrac{3}{2}$]{
	\includegraphics[scale=0.95]{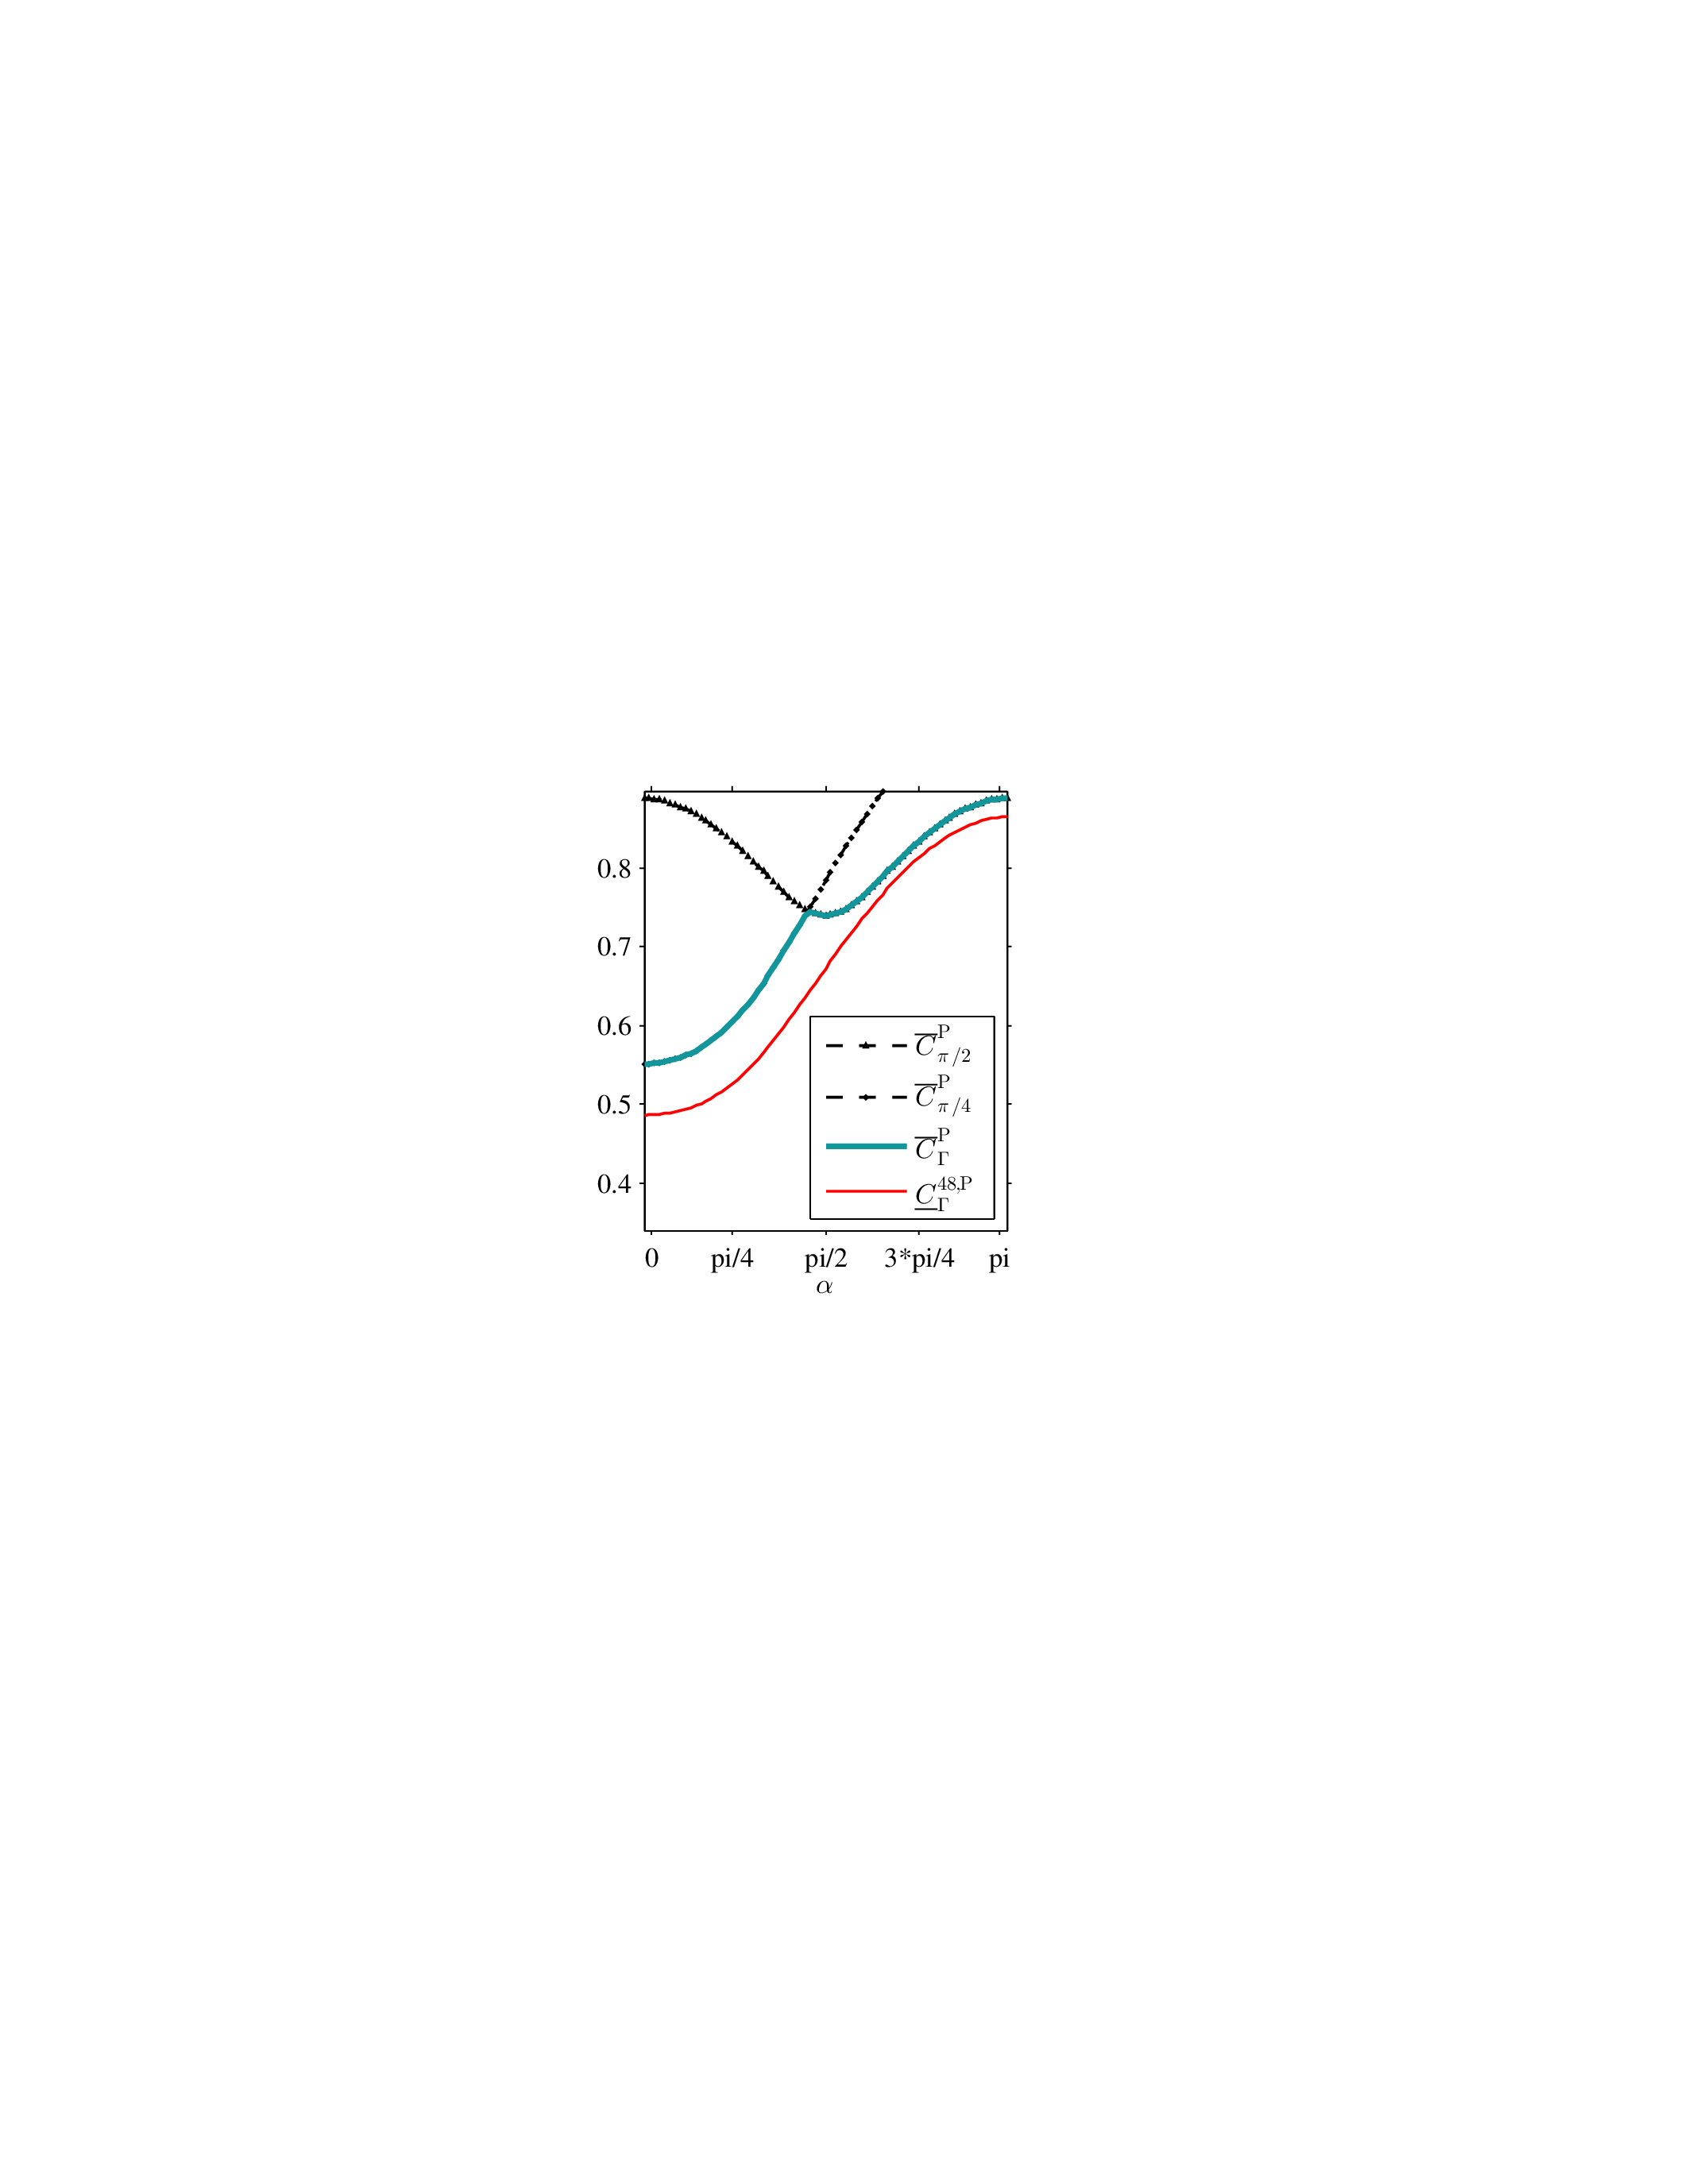}
	\label{fig:2d-cpt-rho-3-2}}
	\caption{Lower and upper bounds  of $\CPT$
	%$\CP = \min \,\{ {\CP}_{\rm I}, {\CP}_{\rm II} \}$ 
	for $\T \in \Rtwo$ (a) $\rho = \tfrac{\sqrt{3}}{2}$ and (b) $\rho = \tfrac{3}{2}$.}
	\label{fig:2d-cpt-no-ref}
\end{figure}
\vskip -10pt
%--------------------------------------------------------------------------------------------%
% \CGT with upper bounds
%--------------------------------------------------------------------------------------------%
\begin{figure}[!ht]
	\centering
	\subfloat[$\rho = \tfrac{\sqrt{3}}{2}$]{
  \includegraphics[scale=0.95]{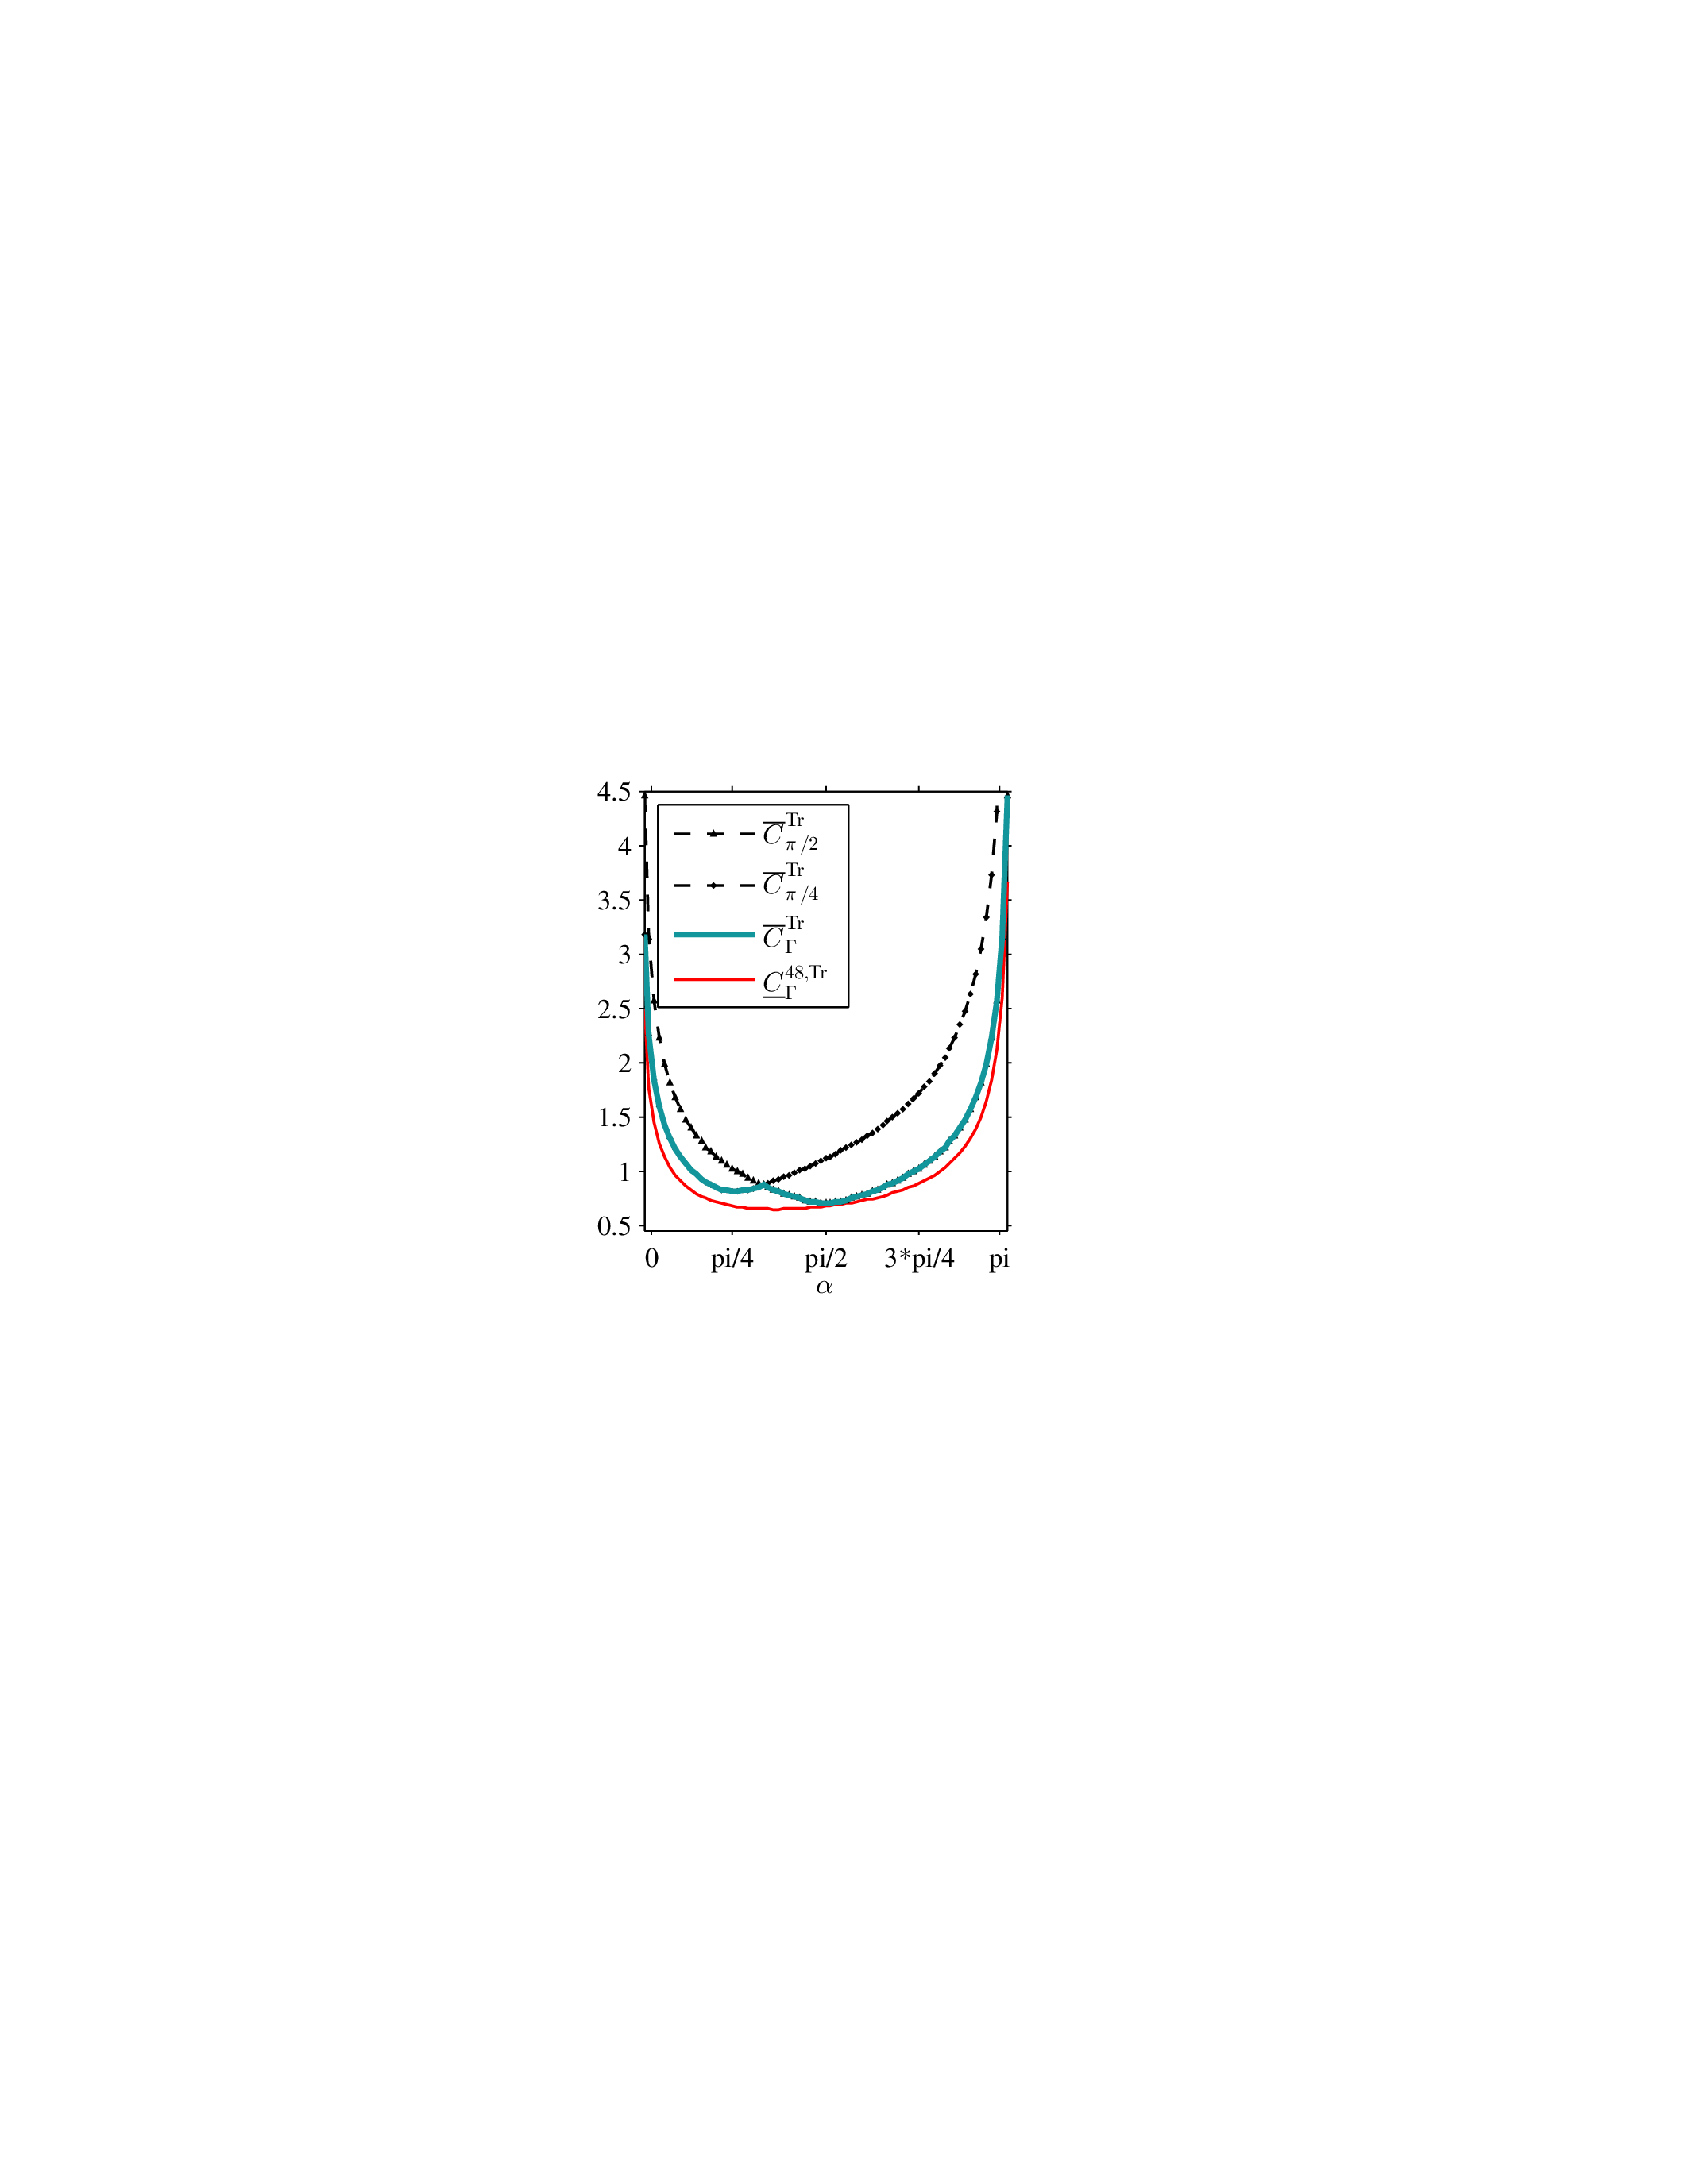}
	\label{fig:2d-cgt-rho-sqrt3-2}}
	\quad
	\subfloat[$\rho = \tfrac{3}{2}$]{
	\includegraphics[scale=0.95]{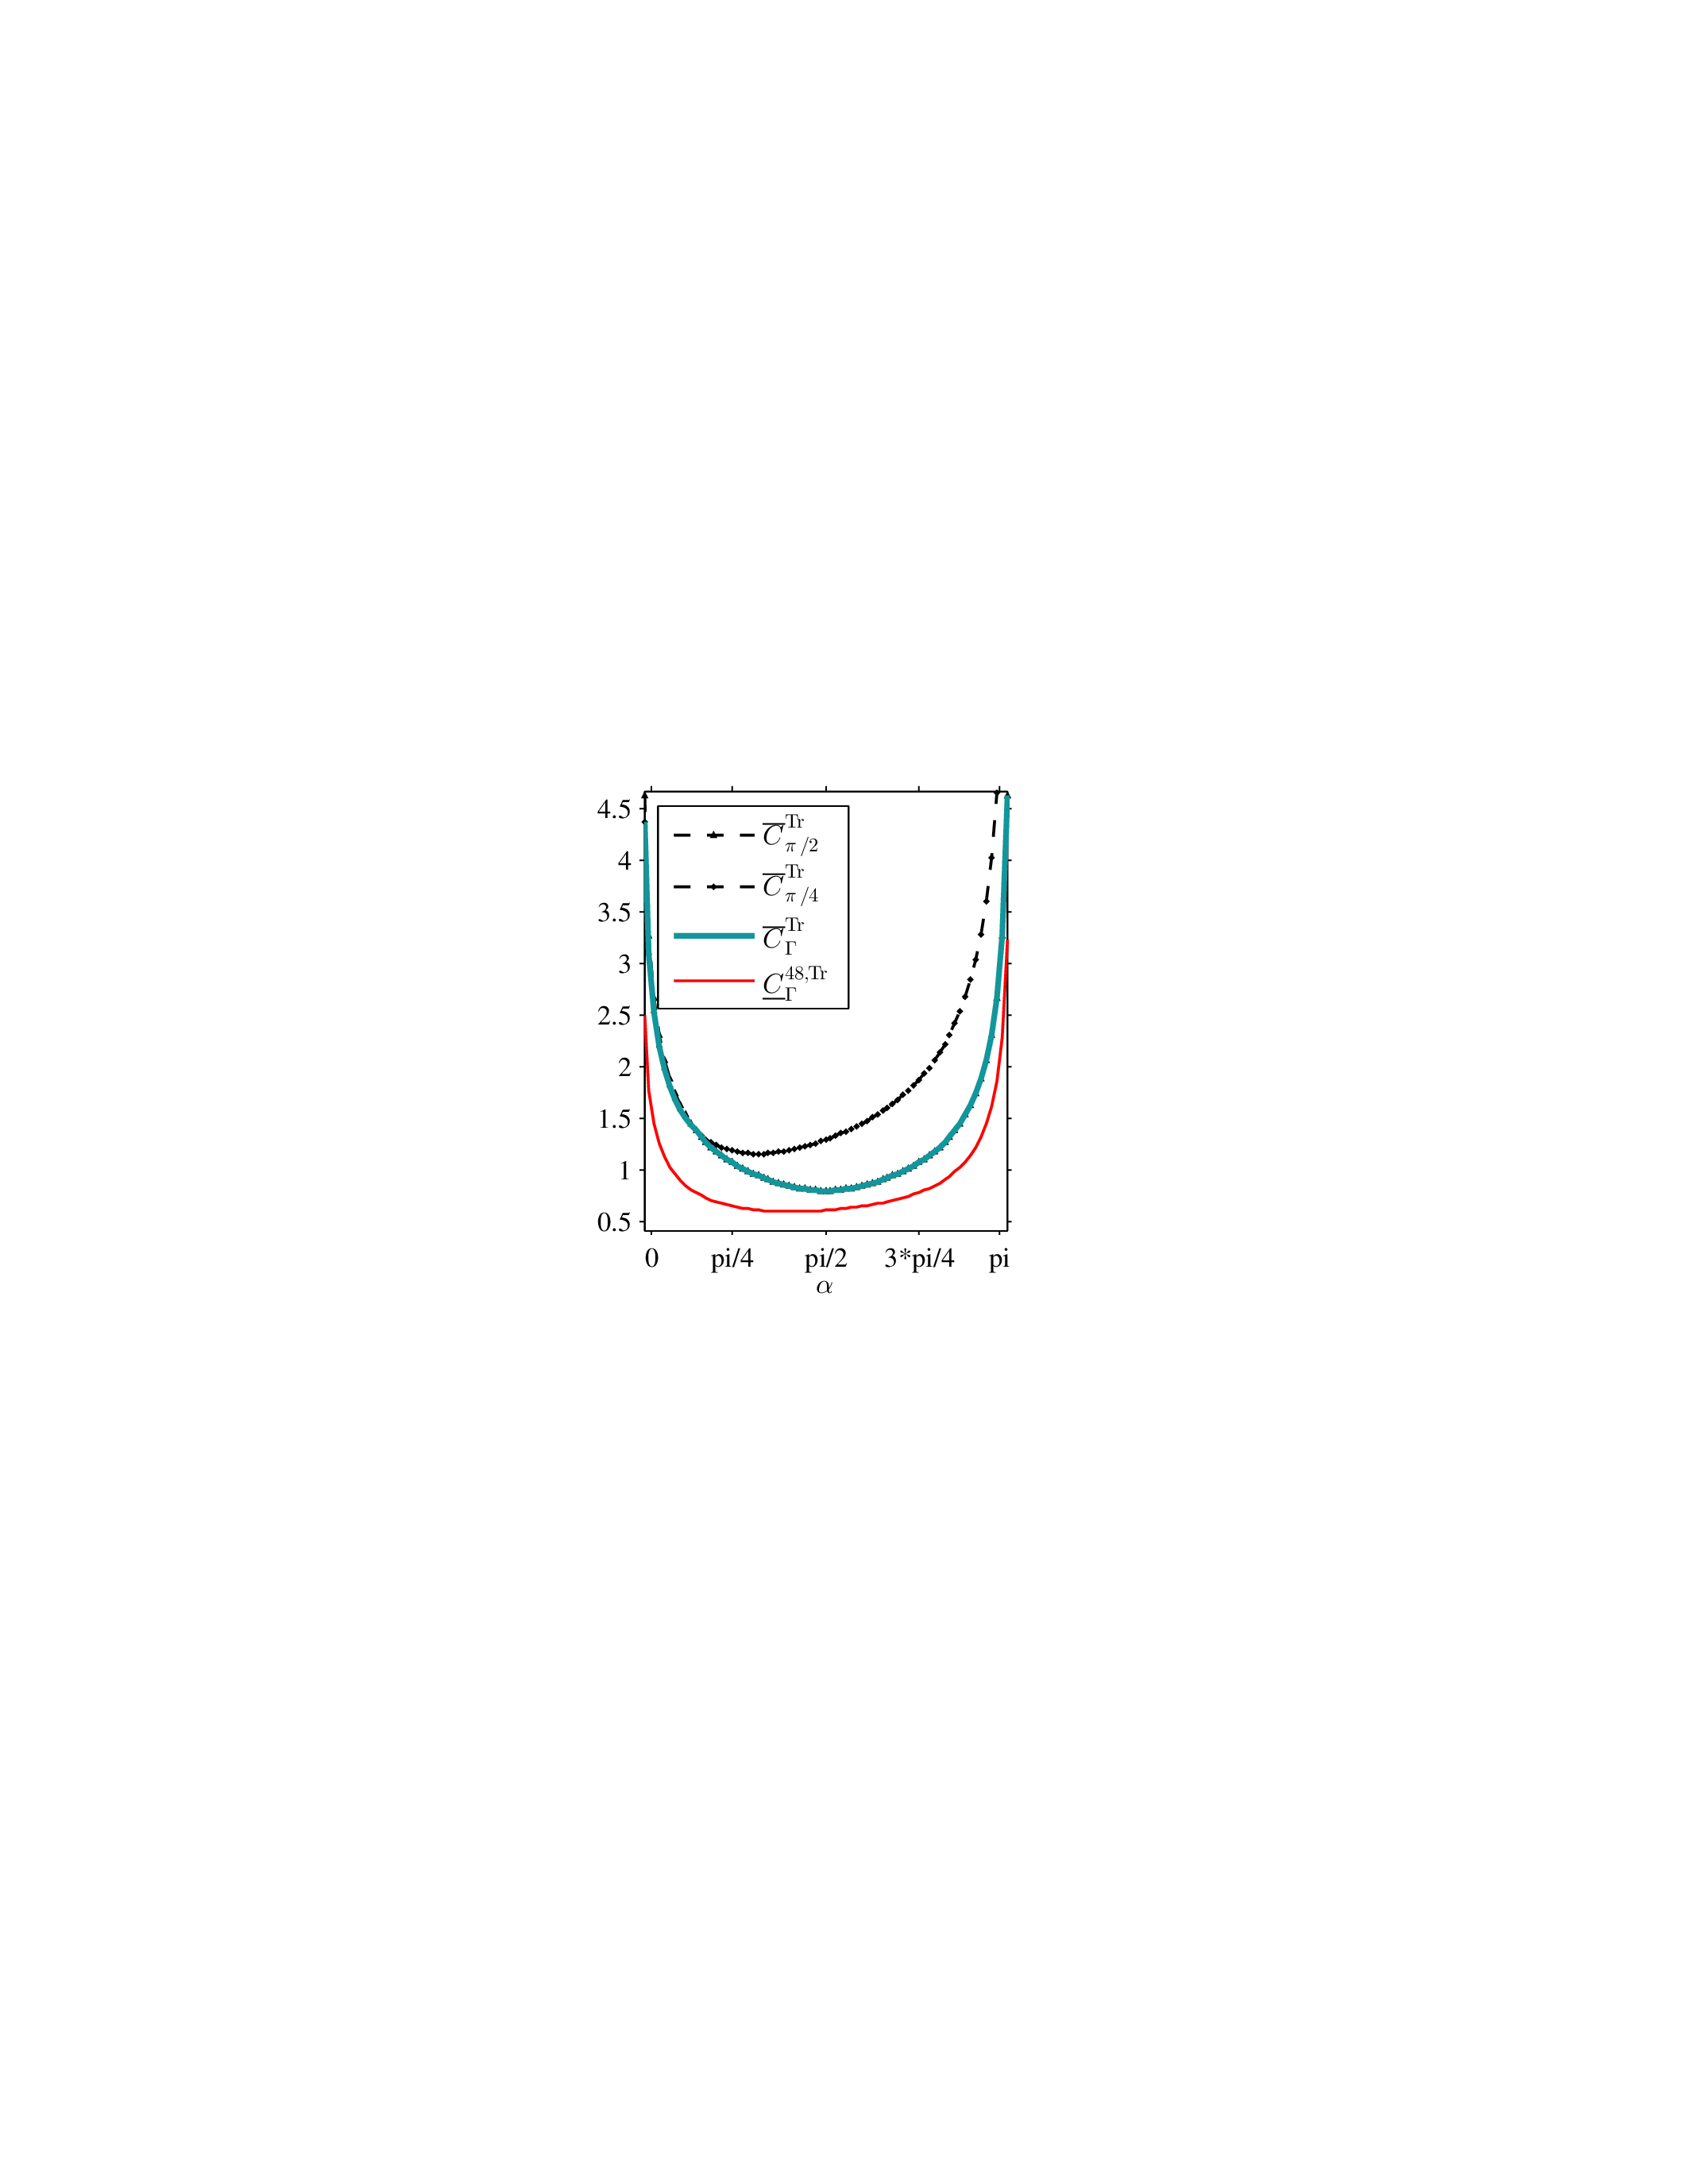}
	\label{fig:2d-cgt-rho-3-2}}
	\caption{Lower and upper bounds  of $\CGT$
	%$\CP = \min \,\{ {\CP}_{\rm I}, {\CP}_{\rm II} \}$ 
	for $\T \in \Rtwo$ (a) $\rho = \tfrac{\sqrt{3}}{2}$ and (b) $\rho = \tfrac{3}{2}$.}
	\label{fig:2d-cgt-no-ref}
\end{figure}
% 
%********************************************************************************************
%rho = 0.71, 1.5
%********************************************************************************************
\begin{figure}[!ht]
	\centering
	\subfloat[$\rho = \tfrac{\sqrt{2}}{2}$]{
	\includegraphics[scale=0.8]{2d-cp-mean-value-on-T-rho-0-70711-h-1-1-power-series}
	\label{fig:cp-rho-sqrt2-2}}\\
	\subfloat[$\rho = 1$]{
	\includegraphics[scale=0.8]{2d-cp-mean-value-on-T-rho-1-h-1-1-power-series}
	\label{fig:cp-rho-1}} \\
	\subfloat[$\rho = \tfrac{3}{2}$]{
	\includegraphics[scale=0.8]{2d-cp-mean-value-on-T-rho-1-5-h-1-1-power-series}
	\label{fig:cp-rho-3-2}
	}
	\caption{$\underline{C}^{48}_{\T}$ with upper and lower bounds 
	with respect to $\alpha$ on $\T$ with (a) $\rho = \tfrac{\sqrt{2}}{2}$ and (b) $\tfrac{3}{2}$.}	
	\label{fig:2d-cp-rho}
\end{figure}

\begin{figure}[!ht]
  \centering
	\includegraphics[scale=0.8]{2d-cp-mean-value-on-T-improved-rho-1-h-1-1-power-series}
	\captionof{figure}{Approximation $\underline{C}^{48}_{\T}$ with improved upper and 
	lower bounds on isosceles $\T$ with respect to $\alpha$.}
	\label{fig:cp-rho-1-improved}
\end{figure}
 
\input{func-cpgamma} 
\input{func-ctrgamma}
\input{switch-func-cp-rho-1}
\input{cpgamma-ctrgamma-with-estimates-3d}
